# Supplementary material for: Training Variational Autoencoders with Buffered Stochastic Variational Inference
Source: arXiv:1902.10294 source file (2019-02-27)
Supplement: Supplementary file 1 [file appendix_old.tex]

\newpage
\appendix

\section{Overly Expressive Amortization Family Hurts Generalization}
\label{app:large_encoder}
In the experiments by \cite{cremer2018inference}, they observed that an overly expressive amortization family increases the test set inference gap, but does not impact the test set log-likelihood. We show in \cref{table:large_encoder} that \cite{cremer2018inference}'s observation is not true in general, and that an overly expressive amortization family can in fact hurt test set log-likelihood. Details regarding the architectures are provided in \cref{app:architecture}.

\input{tables/large_encoder.tex}

%\todo{maybe add a table of the regularizers and types of models (VAE, IWAE), what each regularizer do and how are they affected by the type of model}

\section{Revisiting \cite{im2017denoising}'s Denoising Variational Autoencoder Analysis}\label{app:dvae}

In \cite{im2017denoising}'s Lemma 1, they considered a joint distribution $p_\theta(x, z)$. They introduced an auxiliary variable $z'$ into their inference model (here $z'$ takes on the role of the perturbed input $\tilde{x} = x + \veps$. To avoid confusion, we stick to the notation used in their Lemma) and considered the inference model
\begin{align}
q_\varphi(z \giv z')q_\psi(z' \giv x).
\end{align}
They considered two ways to use this inference model. The first approach is to marginalize the auxiliary latent variable $z'$. This defines the resulting inference model
\begin{align}
q_\phi(z \giv x) = \int q_\varphi(z \giv z')q_\psi(z' \giv x) dz'.
\end{align}
This yields the lower bound
\begin{align}
\L_a = \Expect_{q_\phi(z \giv x)} \brac{\ln \frac{p_\theta(x, z)}{q_\phi(z \giv x)}}.
\end{align}
Next, they considered an alternative lower bound
\begin{align}
\L_b = \Expect_{q_\varphi(z \giv z')q_\psi(z' \giv x)}\brac{\ln \frac{p_\theta(x, z)}{q_\varphi(z \giv z')}}.
\end{align}
\cite{im2017denoising}'s Lemma 1 claims that 
\begin{enumerate}
\item $\L_a$ and $\L_b$ are valid lower bounds of $\ln p_\theta(x)$
\item $\L_b \ge \L_a$.
\end{enumerate}
Using Lemma 1, \cite{im2017denoising} motivated the denoising variational autoencoder by concluding that it provides a tighter bound than marginalization of the noise variable. Although statement 1 is correct, statement 2 is not. Their proof of statement 2 is presented as follows
\begin{align}
\Expect_{q_\varphi(z \giv z')q_\psi(z' \giv x)}\brac{\ln \frac{p_\theta(x, z)}{q_\varphi(z \giv z')}}
&\stackrel{?}{=} \Expect_{q_\phi(z \giv x)}\brac{\ln \frac{p_\theta(x, z)}{q_\varphi(z \giv z')}} \label{eq:step}\\
&= \Expect_{q_\phi(z \giv x)} \brac{\log p_\theta(x, z)} - \Expect_{q_\phi(z \giv x)} \brac{\ln q_\phi(z \giv z')} \\
&\ge \Expect_{q_\phi(z \giv x)} \brac{\log p_\theta(x, z)} - \Expect_{q_\phi(z \giv x)} \brac{\ln q_\phi(z \giv z')} \\
&= \Expect_{q_\phi(z \giv x)} \brac{\ln \frac{p_\theta(x, z)}{q_\phi(z \giv x)}}
\end{align}
We indicate the mistake with $\stackrel{?}{=}$; their proof of statement 2 relied on the assumption that
\begin{align}
\Expect_{q_\varphi(z \giv z')q_\psi(z' \giv x)}\brac{\ln \frac{p_\theta(x, z)}{q_\varphi(z \giv z')}} = \Expect_{q_\phi(z \giv x)}\brac{\ln \frac{p_\theta(x, z)}{q_\varphi(z \giv z')}}.
\end{align}
Crucially, the RHS is ill-defined since it does not take the expectation over $z'$, whereas the LHS explicitly specifies an expectation over $z' \sim q_\psi(z' \giv x)$. This difference, while subtle, invalidates the subsequent steps. If we fix \cref{eq:step} and attempt to see if the rest of the proof still follows, we will find that
\begin{align}
\Expect_{q_\varphi(z \giv z')q_\psi(z' \giv x)}\brac{\ln \frac{p_\theta(x, z)}{q_\varphi(z \giv z')}}
&= \Expect_{q_\phi(z \giv x)} \brac{\log p_\theta(x, z)} 
- \Expect_{q_\varphi(z \giv z')q_\psi(z' \giv x)} \brac{\ln q_\psi(z \giv z')} \\
&\not\ge \Expect_{q_\phi(z \giv x)} \brac{\log p_\theta(x, z)} 
- \Expect_{q_\varphi(z \giv z')q_\psi(z' \giv x)} \brac{\ln q_\phi(z \giv x)}\\
&= \Expect_{q_\phi(z \giv x)} \brac{\ln \frac{p_\theta(x, z)}{q_\phi(z \giv x)}}.
\end{align}
Indeed, the inequality will point the other way since
\begin{align}
\Expect_{q_\varphi(z \giv z')q_\psi(z' \giv x)} \brac{\ln q_\psi(z \giv z') - \ln q_\phi(z \giv x)}
&= \Expect_{q_\psi(z' \giv x)}\Expect_{q_\varphi(z \giv z')} \ln \frac{q_\varphi(z \giv z')}{q_\phi(z \giv x)} \\
&= \Expect_{q_\psi(z' \giv x)}\KL{q_\varphi(z \giv z')}{q_\phi(z \giv x)} \\
&\ge 0 \implies \\
-\Expect_{q_\varphi(z \giv z')q_\psi(z' \giv x)} \brac{\ln q_\psi(z \giv z')} &\le 
-\Expect_{q_\varphi(z \giv z')q_\psi(z' \giv x)} \brac{\ln q_\phi(z \giv x)}.
\end{align}
Their conclusion that marginalizing over the noise variable results in a looser bound is thus incorrect. In the text (beneath \cite{im2017denoising} Eq. (11)), they further implied that the denoising VAE and standard VAE objectives are not comparable. We show in \cref{prop:strength} that the denoising VAE objective is in fact a lower bound of the standard VAE objective.

\section{Importance-Weighted Stochastic Variational Inference}\label{app:iwsvi}

\input{figures/iwsvi.tex}

We propose a simple method to approximate the marginal $\ln p_\theta(x)$. A common approach for approximating the log marginal is the IWAE-$5000$ \cite{burda2015importance,sonderby2016ladder,li2016renyi,tomczak2017vae}, which proposes to compute $\L_{5000}(x\scolon \theta,\phi)$ where
\begin{align}
\ln p_\theta(x) \ge \L_k(x \scolon \theta, \phi) 
= \Expect_{z_1\ldots z_k \sim q_\phi(z \giv x)} \paren{\ln \frac{1}{k} \sum_{i=1}^k \frac{p_\theta(x, z^{(i)})}{q_\phi(z^{(i)} \giv x)}}.
\end{align}

However, this approach relies on the learned inference model $q_\phi(z \giv x)$, which might overfit to the training set. To address this issue, we propose to perform importance-weighted stochastic variational inference (IW-SVI)
\begin{align}
\ln p_\theta(x) \ge \L_k(x \scolon \theta, q^*_{x,\ell}) &= \Expect_{z_1\ldots z_k \sim q^*_{x,\ell}(z)} \paren{\ln \frac{1}{k} \sum_{i=1}^k \frac{p_\theta(z \giv x)}{q^*_{x,\ell}(z)}}, \\
\text{where } q^*_{x,\ell}  &= \argmax_{q \in \Q} \L_\ell(x \scolon \theta, q).\label{eq:optimize}
\end{align}
The optimization in \cref{eq:optimize} is approximate with $T$ gradient steps. As $k$ and $\ell$ increase, the approximation will approach the true log-likelihood. We approximate log-likelihood over the entire test set using $\Expect_{\hat{p}_\text{test}(x)}\L_k(p_\theta, q^*_{x,\ell} \scolon x)$. To reduce speed and memory cost during the per-sample optimization in \cref{eq:optimize},  we use a large $k = 5000$ but smaller $\ell = 8$, and approximately solved the optimization problem using $T=3000$ gradient steps. In comparison to IWAE-$5000$, we consistently observe significant improvement in the log-likelihood approximation. IW-SVI provides a simple alternative to Annealed Importance Sampling, requiring minimal modification to any existing IWAE-$k$ implementation.

\section{Are High Signal-to-Noise Ratio Gradients Necessarily Better?}\label{app:snr}

Our paper shares a similar high level message with a recent study by \cite{rainforth2018tighter}: that approximating maximum likelihood training is not necessarily better. However, we approach this message in very different ways. \cite{rainforth2018tighter} observed that importance sampling weakens the signal-to-noise ratio of the gradients used to update the amortized inference model. In response, they proposed to increase this ratio by increasing the number of Monte Carlo samples $m$ used to estimate the expectation in \cref{eq:vae}. Under a fixed budget of $T \ge mk$ (where $k$ is the number of importance samples and $m$ is the number of Monte Carlo samples), they observed that it may be desirable to trade off $k$ in order to increase $m$. Given an infinite budget, however, \cite{rainforth2018tighter}'s hypothesis would still conclude to increase $k$ as much as possible in order to approximate maximum likelihood training.

In contrast, we argue that it may be inherently desirable to regularize the maximum likelihood objective, and that amortized inference regularization is an effective means of doing so. From the perspective of generalization, it is also worth wondering whether high signal-to-noise ratio gradients are necessarily better. The desirability of noisy gradients for improving generalization is an active area of research \cite{smith2018sgd,dinh2017sharp,masters2018revisiting,zhang2016understanding}, and an extensive investigation of the role of gradient stochasticity in regularizing the amortized inference model is beyond the scope of our paper. To encourage future exploration in this direction, we show in \Cref{fig:snr_analysis} that the effect of gradient stochasticity is non-negligible. For the standard VAE, we observed that increasing $m$ can cause the model to overfit (on the amortized ELBO objective) over the course of training. Interestingly, we observed that DVAE does not experience this overfitting effect, suggesting that AIR is robust to larger values of $m$.

\input{figures/snr_analysis.tex}

\clearpage
\section{Experimental Details}\label{app:architecture}
%\rs{Talk about early stopping and hyperparamter tuning}
%\rs{Talk about usage of standard error of mean}

\textbf{Datasets.} We carried out experiments on the static MNIST, static OMNIGLOT, and Caltech 101 Silhouettes datasets. OMNIGLOT was statically binarized at the beginning of training via random sampling using the pixel real-values as Bernoulli parameters. Training, validation, and test split sizes are provided in \cref{table:datasets}. The MNIST validation set was created by randomly holding out $10000$ samples from the original $60000$-sample training set. The OMNIGLOT validation set was similarly created by randomly holding out $1345$ samples from the original $24345$-sample training set. 

\input{tables/datasets.tex}

\textbf{Training parameters.} Important training parameters are provided in \cref{table:architectures}. We used the Adam optimizer and exponentially decayed the initial learning rate according to the formula
\begin{align}
\alpha_t = \alpha_0 \cdot (0.1)^{\frac{t}{T - 1}},
\end{align}
where $t \in \seta{0, \ldots, T - 1}$ is the current iteration and $T$ is the total number of iterations. Early-stopping is applied according to IWAE-$5000$ evaluation on the validation set. 

\input{tables/architectures.tex}

\textbf{Regularization strength tuning.} The denoising and weight normalization regularizers have hyperparameters $\sigma$ and $H$ respectively. See \cref{table:strengths} for hyperparameter search space details. We performed a basic grid search and tuned the regularization strength hyperparameters based on the validation set.

\input{tables/strengths.tex}

\clearpage
\section{Proofs}

\textbf{Remark.} Some of the proofs mention the notion of an infinite capacity $\F$, $\G$ or $\Q$. To clarify, we say that $\F$ has infinite capacity if it is the set of all possible functions that map from $\X$ to $\Q$. Analogously, $\G$ has infinite capacity if it is the set of all possible functions that map from $\Z$ to $\P$. We say that $\Q$ has infinite capacity if it is the set of all possible distributions over the space $\Z$.

\PropKernel*
\begin{proof}
Define $\tilde{x} = x + \veps$ and 
$\phat(x, \tilde{x}) = \phat(x)\Normal(\tilde{x} \giv x, \sigma\I)$. Rewrite the objective as
\begin{align}
R(\theta \scolon \sigma) &= \min_{f \in \F(\Q)}\Expect_{\phat(x, \tilde{x})}\brac{\KL{f(\tilde{x})}{p_\theta(z \giv x)}}\\
&\ge \Expect_{\phat(\tilde{x})}\min_{q \in \Q}\Expect_{\phat(x \giv \tilde{x})}\brac{\KL{q(z)}{p_\theta(z \giv x)}}.
\end{align}
Recall that $\F$ has infinite capacity. This lower bound is tight since we can select $f^*_\sigma \in \F$ such that
\begin{align}
f^*_\sigma(\tilde{x}) = \argmin_{q \in \Q} \Expect_{\phat(x \giv \tilde{x})} \KL{q(z)}{p_\theta(z \giv x)}.\label{eq:prekernel}
\end{align}
Reexpressing \cref{eq:prekernel} by expanding $\phat(x \giv \tilde{x})$ yields \cref{eq:kernel}.
\end{proof}

\ThmSmooth*
\begin{proof} 
Proof provided in two parts.

\textbf{Part 1.} The Kullback-Leibler divergence can be represented as a Bregman divergence associated with the strictly convex log-partition function $A$ of the minimal exponential family as follows
\begin{align}
\KL{\eta}{\eta^{(i)}} = d_A(\eta^{(i)}, \eta) = A(\eta^{(i)}) - A(\eta) - \nabla A(\eta)^\top(\eta^{(i)} - \eta).
\end{align}
Proposition 1 from \cite{banerjee2005clustering} shows that that for any convex combination weights $\set{w_i}, \sum_{i=1}^n w_i = 1$, the minimizer of a weighted average of Bregman divergences is 
\begin{align}
\sum_{i=1}^n w_i x_i = \argmin_{y \in \Omega} \sum_{i=1}^n w_i d_A(x_i, y).
\end{align}
It thus follows that 
\begin{align}
f^*_\sigma(x) 
&= \argmin_{\eta \in \Omega} \sum_{i=1}^n w_\sigma(x, x^{(i)}) \cdot \KL{\eta}{\eta^{(i)}}\\
&= \argmin_{\eta \in \Omega} \sum_{i=1}^n w_\sigma(x, x^{(i)}) \cdot d_A(\eta^{(i)}, \eta) \\
&= \sum_{i=1}^n w_\sigma(x, x^{(i)}) \cdot \eta^{(i)}.
\end{align}
\textbf{Part 2.} We will write the derivative $\nabla_{x} f^*_\sigma(x)$ in matrix form by the following notation
\begin{align*}
\nabla_x W_\sigma(x) &= \left( \begin{array}{ccc} \nabla_x w_\sigma(x, x^{(1)}) & \cdots & \nabla_x w_\sigma(x, x^{(m)}) \end{array} \right) \\
M &= \left( \begin{array}{ccc} \eta^{(1)} & \cdots & \eta^{(m)} \end{array} \right) 
\end{align*}
where we also suppose input space $x$ is $n$-dimensional, latent parameter space $\Omega$ is $d$-dimensional, and there are $m$ training examples.
%\sj{To check during final pass that these notations are consistent} 
Then
\[ \nabla_x f^*_\sigma(x) = M \nabla_x W_\sigma(x)^T  \]
Let $\lVert \cdot \rVert_1$ be the induced 1-norm for matrices, then by the sub-multiplicative property
\begin{align*}
\lVert \nabla_x f^*(x) \rVert_1 \leq \lVert M \rVert_1 \lVert \nabla_x W_\sigma(x)^T \rVert_1
\end{align*}
Since $\lVert M \rVert_1$ is a constant with respect to $\sigma$, we only have to bound $\lVert \nabla_x W_\sigma(x)^T \rVert_1$. To do this we study the derivative of $\nabla_x w_\sigma(x, x^{(i)})$, where
\begin{align*}
\nabla_x w_\sigma(x, x^{(i)}) &= \nabla_x \frac{K_\sigma(x, x^{(i)})}{\sum_j K_\sigma(x, x^{(j)})} \\
&= \frac{ K(x, x^{(i)})\frac{x^{(i)}-x}{\sigma^2} \sum_j K_\sigma(x, x^{(j)}) + K(x, x^{(i)})\sum_j  K(x, x^{(j)})\frac{x-x^{(j)}}{\sigma^2}}{(\sum_j K_\sigma(x, x^{(j)}))^2} \\
&= \frac{ K(x, x^{(i)}) \sum_j K_\sigma(x, x^{(j)}) \frac{x^{(i)} - x^{(j)}}{\sigma^2}}{(\sum_j K_\sigma(x, x^{(j)}))^2} 
\end{align*}
Let $|\cdot|$ denote taking element-wise absolute value, and $x \leq^* y$ denotes for all elements of the vector $|x_i| \leq |y_i|$. By Cauchy inequality and $\lVert \cdot \rVert_2 \leq \lVert \cdot \rVert_1$ we have
\begin{align*}
\nabla_x w_\sigma(x, x^{(i)}) &\leq^* \frac{K(x, x^{(i)}) \sum_j K(x, x^{(j)}) \sum_j |x^{(i)} - x^{(j)}|}{\sigma^2 (\sum_j K_\sigma(x, x^{(j)}))^2}
\leq^* \frac{1}{\sigma^2}\sum_j |x^{(i)} - x^{(j)}|
\end{align*}
Therefore 
\begin{align*}
\sup_x \lVert \nabla_x w_\sigma(x, x^{(i)}) \rVert_1 = O(1/\sigma^2)
\end{align*}
% \begin{align*}
% \sup_x \lVert \nabla_x w_\sigma(x, x^{(i)}) \rVert_1 &= \sup_x \left\lVert \nabla_x \frac{K_\sigma(x, x^{(i)})}{\sum_j K_\sigma(x, x^{(j)})} \right\rVert_1  &= \sup_x \lVert \nabla_x e^{-\frac{\lVert x \rVert^2}{2\sigma^2}} \rVert_1 
% = \sum_{i=1}^n \sup_x \frac{\partial e^{-x_i^2/(2\sigma^2)}}{\partial x_i} 
% \end{align*}
% %\sj{one more thing to do: taking into consideration the normalization}
% Taking first and second order derivatives we have
% \begin{align*}
% \frac{\partial e^{-x_i^2/2\sigma^2}}{\partial x_i} &= -x_i/\sigma^2 e^{-x_i^2/(2\sigma^2)} \\
% \frac{\partial^2 e^{-x_i^2/2\sigma^2}}{\partial x_i^2} &\propto (x_i^2 - \sigma^2) e^{-x_i^2/(2\sigma^2)} 
% \end{align*}
% The supremum for the first order derivative is achieved at $x_i = - \sigma$, so
% \begin{align*}
% \sup_x \lVert \nabla_x w_\sigma(x, x^{(i)}) \rVert_1 &= \frac{d e^{-1/2}}{\sigma} 
% \end{align*}
This gives us a bound on the matrix 1-norm
\begin{align*}
\sup_x \lVert \nabla_x W_\sigma(x)^T \rVert_1 \leq \sup_x \sqrt{mn} \lVert \nabla_x W_\sigma(x)^T \rVert_\infty = \sqrt{mn} \sup_x \max_{i=1}^{n} \lVert \nabla_x w_\sigma(x, x^{(i)}) \rVert_1 = O(1/\sigma^2) 
\end{align*}
Because both $\Omega$ and $\mathcal{X}$ are convex sets, this implies the following Lipschitz property
\[ \frac{\lVert f^*(x_1) - f^*(x_2) \rVert_1}{\lVert x_1 - x_2 \rVert_1} \leqslant \sup_x \lVert \nabla_x f^*(x) \rVert_1 = O(1/\sigma^2)  \]
\end{proof}

\PropStrength*
\begin{proof}
Proof is provided in two parts.

\textbf{Part 1.} Recall that $R$ is always non-negative. Since there exists $\theta \in \Theta$ such that $p_\theta(x, z) = p_\theta(z)p_\theta(x)$, and $f \in \F$ such that $f(x) = p_\theta(z)$, then $\min_\theta R(\theta\scolon \sigma) = 0$ for any choice of $\sigma$. 

\textbf{Part 2.} Let $\veps_1 \sim \Normal(\0, \sigma_1\I)$, $\veps_2 \sim \Normal(\0, \sigma_2\I)$, and $\veps_\delta = \Normal(\0, (\sigma_1 - \sigma_2)\I)$. Then
\begin{align}
R(\theta\scolon \sigma_1)
&= \min_{f \in \F} \Expect_{\veps_1}\Expect_{\phat(x)}\brac{\KL{f(x + \veps_1)}{p_\theta(z \giv x)}}\\
&= \min_{f \in \F} \Expect_{\veps_\delta}\Expect_{\veps_2}\Expect_{\phat(x)}\brac{\KL{f(x + \veps_\delta + \veps_2)}{p_\theta(z \giv x)}}\\
&\ge \Expect_{\veps_\delta}\min_{f \in \F} \Expect_{\veps_2}\Expect_{\phat(x)}\brac{\KL{f(x + \veps_\delta + \veps_2)}{p_\theta(z \giv x)}}.
\end{align}
Since $\F$ is closed under input translation,
\begin{align}
\Expect_{\veps_\delta}\min_{f \in \F} \Expect_{\veps_2}\Expect_{\phat(x)}\brac{\KL{f(x + \veps_\delta + \veps_2)}{p_\theta(z \giv x)}} = R(\theta \scolon \veps_2).
\end{align}
It thus follows that $R(\theta \scolon \sigma_1) \ge R(\theta \scolon \sigma_2)$ for all $\theta \in \Theta$.
\end{proof}

\PropDecoder*
\begin{proof}
For a given inference model $q(z \giv x)$, the optimal generator maximizes the objective
\begin{align}
\max_{g \in \G} \Expect_{\phat(x)}\Expect_{q(z \giv x)} \brac{\ln g(z)(x)} &= \max_{g \in \G} \Expect_{q(x, z)} \brac{\ln g(z)(x)}.\label{eq:g}\\
&= \max_{g \in \G} \Expect_{q(x, z)} \brac{\ln p_{g(z)}(x)} \\&\le \Expect_{q(z)} \max_{p \in \P}\Expect_{q(x \giv z)} \ln p(x)\\
&= \Expect_{q(z)} \max_{\mu \in \M}\Expect_{q(x \giv z)} \ln p_\mu(x),
\end{align}
where $p_\mu$ denotes the distribution $p \in \P$ with associate mean parameter $\mu$. This inequality is tight since we can select $g^* \in \G$ such that
\begin{align}
g^*(z) = \argmax_{\mu \in \M}\Expect_{q(x \giv z)} \ln p_\mu(x).
\end{align}
Recall that the maximum likelihood and maximum entropy solutions are equivalent for an exponential family. From the moment-matching condition of maximum entropy, it follows that
\begin{align}
g^*(z) &= \argmax_{\mu \in \M}\Expect_{q(x \giv z)} \ln p_\mu(x) \\
&= \Expect_{q(x \giv z)} \brac{T(x)} \\
&= \sum_{i=1}^n q(x^{(i)} \giv z) \cdot T(x^{(i)})\\
&= \sum_{i=1}^n \paren{\frac{q(z \giv x^{(i)})}{\sum_j q(z \giv x^{(j)})} \cdot T(x^{(i)})}.
\end{align}
\end{proof}

\PropIWAE*
\begin{proof}
Proof is provided in two parts.

\textbf{Part 1.} The relevant assumptions are that there exists $\theta \in \Theta$ such that $p_\theta(x, z) = p_\theta(z)p_\theta(x)$, and $f \in \F_H$ such that $f(x) = p_\theta(z)$. Note that $R_k$ is always non-negative. It follows readily that $\min_\theta R_k(\theta\scolon \sigma, \F_H) = 0$ for any choice of $k$. 

\textbf{Part 2.} We define $\L_k$ as
\begin{align}
\L_k &= \Expect_{\phat(x)} \ln p_\theta(x) - R_k(\theta \scolon \sigma, \F_H) \\
&= \max_{f \in \F_H} \Expect_{\phat(x)}\Expect_{\veps} \Expect_{z_1\ldots z_k \sim f(x + \veps)}\brac{\ln \frac{1}{k} \sum_{i=1}^k \frac{p_\theta(x, z_i)}{f(x + \veps)(z_i)}}.
\end{align}
It suffices to show that $\L_{k} \ge \L_{m}$ when $k \ge m$.
We adapt the proof from \cite{burda2015importance}'s Theorem 1 as follows. Let $|I| = m$ denote a uniformly distributed subset of distinct indices from $\seta{1, \ldots, k}$. For any choice of $f \in \F_H$, the following inequality holds
\begin{align}
&\Expect_{\phat(x)}\Expect_{\veps} \Expect_{z_1\ldots z_k \sim f(x + \veps)}\brac{\ln \frac{1}{k} \sum_{i=1}^k \frac{p_\theta(x, z_i)}{f(x + \veps)(z_i)}}\\
&= \Expect_{\phat(x)}\Expect_{\veps} \Expect_{z_1\ldots z_k \sim f(x + \veps)}\brac{\ln \Expect_{I=\seta{i_1\ldots i_m}}\brac{\frac{1}{m} \sum_{j=1}^m \frac{p_\theta(x, z_{i_j})}{f(x + \veps)(z_{i_j})}}}\\
&\ge \Expect_{\phat(x)}\Expect_{\veps} \Expect_{z_1\ldots z_k \sim f(x + \veps)}\Expect_{I=\seta{i_1\ldots i_m}}\brac{\ln \frac{1}{m} \sum_{j=1}^m \frac{p_\theta(x, z_{i_j})}{f(x + \veps)(z_{i_j})}}\\
&= \Expect_{\phat(x)}\Expect_{\veps} \Expect_{z_1\ldots z_m \sim f(x + \veps)}\brac{\ln \frac{1}{m} \sum_{i=1}^m \frac{p_\theta(x, z_{i})}{f(x + \veps)(z_{i}))}}.
\end{align}
It thus follows that $\L_k \ge \L_m$.
\end{proof}

%\rs{Check that I don't have $\F_K$. Check that notation is consistent. Check for spelling and grammar. Check that all proofs are provided. Decide if Appendix A should be mentioned in main text. Check table formatting. Check if plots are consistent with numbers---eyeball. Flesh out missing definitions (e.g. what is $i_m$) in IWAE proof.}
